# Supplementary material for: TopicBERT for Energy Efficient Document Classification
Source: arXiv:2010.16407 source file (2020-10-15)
Supplement: Supplementary file 1 [file emnlp2020_supplementary.pdf]

# Supplementary Material: TopicBERT for Energy Efficient Document Classification

Anonymous EMNLP submission

## A $CO_2$ : Carbon footprint estimation

See Lacoste et al., (2019) and <https://mlco2.github.io/impact/> for details about estimation of carbon footprint calculation:

$CO_2 = \text{Power consumption} \times \text{Time in hours} \times \text{Carbon produced by local power grid}$

$CO_2 = 0.07 \text{ kW} \times \text{Time in hours} \times 0.61 \times 1000 \text{ gram eq. CO}_2/\text{kWh}$

$CO_2 = 0.07 \text{ kW} \times \text{Time in hours} \times 0.61 \times 1000 \times 0.00220462 \text{ lbs eq. CO}_2/\text{kWh}$

where, Power consumption = 0.07KW for NVIDIA Tesla T4 16 GB Processor; Carbon produced by local power grid = 0.61 kg  $CO_2$ /kWh.

In Figure 1, we run BERT for different sequence lengths (32, 64, 128, 526 and 512) with batch-size=4 to estimate  $CO_2$  and GPU-memory consumed. We run 15 epochs and compute run-time (time in hours) over the different sequence lengths, and therefore, use the above  $CO_2$  formulation to estimate carbon footprint in gram eq.

For Table 1, we estimate  $CO_2$  for document classification tasks (BERT fine-tuning) considering 512 sequence length. We first estimate the frequency of BERT fine-tuning in terms of research activities and/or its application beyond. We estimate the following items:

1. Number of of scientific papers based on BERT = 5532 (number of BERT citations to date: 01, June 2020)

2. conference acceptance rate: 25% (i.e., 4 times the original number of submissions or research/application beyond the submissions)

3. average number of datasets used = 5

4. Average run-time of 15 epochs in fine-tuning BERT over 5000 documents (Reuters8-sized data) of maximum 512 sequence length = 12 hours on the hardware-type used

Therefore,

$CO_2 \text{ estimate in fine-tuning BERT} = 0.07 \times$

| Dataset              | Train<br>#docs | Dev<br>#docs | Test<br>#docs | $Z$  | $L$ | $N$ | $b$ |
|----------------------|----------------|--------------|---------------|------|-----|-----|-----|
| Reuters8             | 4.9k           | 0.5k         | 2.1k          | 4813 | 8   | 512 | 4   |
| Imdb                 | 20k            | 5k           | 25k           | 6823 | 2   | 512 | 4   |
| 20NS                 | 9.9k           | 1k           | 7.4k          | 4138 | 20  | 512 | 4   |
| AGNews               | 118k           | 2k           | 7.6k          | 5001 | 4   | 128 | 32  |
| Ohsumed <sup>†</sup> | 24k            | 3k           | 2.9k          | 4553 | 20  | 512 | 4   |

Table 1: Preprocessed data statistics: #docs  $\rightarrow$  number of documents, k  $\rightarrow$  thousand,  $Z \rightarrow$  vocabulary size of NVDM,  $L \rightarrow$  total number of unique labels,  $N \rightarrow$  sequence length used for BERT fine-tuning,  $b \rightarrow$  batch-size used for BERT fine-tuning, (<sup>†</sup>)  $\rightarrow$  multi-labeled dataset

$$(5532 \times 4 \times 5) \times 12 \times 0.61 \text{ kg eq.} = 56,692 \times 2,20462 \text{ lbs eq} = 124,985 \text{ lbs eq.}$$

## B Data statistics and preprocessing

Table 1 shows data statistics of 5 datasets used in complementary + finetuning evaluation of our proposed *TopicBERT* model via Document Classification task. 20NewsGroups (20NS), Reuters8, AG-news are *news* domain datasets, whereas Imdb and Ohsumed datasets belong to *sentiment* and *medical* domains respectively. For NVDM component, we preprocess each dataset and extract vocabulary  $Z$  as follows: (a) tokenize documents into words, (b) lowercase all words, (d) remove stop words<sup>1</sup>, and (c) remove words with frequency less than  $F_{min}$ . Here,  $F_{min} = 100$  for large datasets i.e., Imdb, 20NS, AGnews and Ohsumed, whereas  $F_{min} = 10$  for Reuters8 which is a small dataset.

## C Experimental setup

Table 2 and 3 shows hyperparameter settings of NVDM and BERT components of our proposed *TopicBERT* model for document classification task. We initialize BERT component with pretrained

<sup>1</sup>we use NLTK tool to remove stopwords

BERT-base model released by Devlin et al. (2019). Fine-tuning of *TopicBERT* is performed as follows: (1) perform pretraining of NVDM component, (2) initialize *BERT* component with BERT-base model, (3) perform complementary + efficient fine-tuning, for 15 epochs, using joint loss objective:

$$\mathcal{L}_{TopicBERT} = \alpha \log p(y = y_i | \mathcal{D}) + (1 - \alpha) \mathcal{L}_{NVDM}$$

where,  $\alpha \in \{0.1, 0.5, 0.9\}$ .

For CNN, we follow the experimental setup of Kim (2014).

| Hyperparameter                          | Value(s)             |
|-----------------------------------------|----------------------|
| Learning rate                           | <u>0.001</u> , 0.05  |
| Hidden size ( $H$ )                     | <u>256</u> , 128     |
| Batch size ( $b$ )                      | 4, 32                |
| Non-linearity ( $g$ )                   | sigmoid              |
| Sampling frequency of $\mathbf{h}_{TM}$ | 5, <u>10</u>         |
| Number of topics ( $K$ )                | 50, <u>100</u> , 200 |

Table 2: Hyperparameters search and optimal settings for NVDM component of *TopicBERT* used in the experimental setup for document classification task.

| Hyperparameter                      | Value(s)                              |
|-------------------------------------|---------------------------------------|
| Learning rate*                      | 2e-5                                  |
| Hidden size ( $H_B$ )               | 768                                   |
| Batch size ( $b$ )                  | [4, 32]                               |
| Non-linearity*                      | gelu                                  |
| Maximum sequence length ( $N$ )     | [512, 256, 128, 64, 32 <sup>‡</sup> ] |
| Number of attention heads*          | 12                                    |
| Number of encoder layers* ( $n_l$ ) | 12                                    |
| Vocabulary size*                    | 28996                                 |
| Dropout probability*                | 0.1                                   |
| $\alpha$                            | [0.1, 0.5, <u>0.9</u> ]               |

Table 3: Hyperparameters search and optimal settings for BERT component of *TopicBERT* used in the experimental setup for document classification. <sup>†</sup> → additional hyperparameter introduced for joint modeling in *TopicBERT*, <sup>‡</sup> →  $N = 32$  is only used for AGnews dataset, (\*) → hyperparameter values taken from pretrained BERT-base model released by Devlin et al. (2019)

## D Results of TopicBERT for AGnews

Table 4 shows gains in *performance* and *efficiency* of *TopicBERT* vs *BERT* for AGnews dataset. *Top-*

|                    | Models         | AGnews               |                |                |                |                |
|--------------------|----------------|----------------------|----------------|----------------|----------------|----------------|
|                    |                | F1                   | Rtn            | $T_{epoch}$    | T              | $CO_2$         |
| baselines          | CNN            | 0.916 ± 0.000        | 97.447%        | 0.131          | 0.921          | 393.25         |
|                    | BERT-Avg       | 0.903 ± 0.000        | 96.064%        | -              | 0.075          | 3.20           |
|                    | BERT-Avg + DTR | 0.913 ± 0.000        | 97.128%        | -              | 0.105          | 4.48           |
|                    | DistilBERT-x   | 0.941 ± 0.001        | 100.10%        | <b>0.491</b>   | <b>7.361</b>   | <b>314.31</b>  |
|                    | BERT-x         | 0.940 ± 0.001        | 100.00%        | 0.952          | 14.281         | 609.80         |
| proposal           | TopicBERT-128  | 0.942 ± 0.003        | 100.21%        | 1.004          | 15.065         | 643.27         |
|                    | TopicBERT-64   | <b>0.943</b> ± 0.002 | <b>100.31%</b> | <u>0.723</u>   | <u>10.838</u>  | <u>462.78</u>  |
|                    | TopicBERT-32   | 0.938 ± 0.001        | 99.78%         | 0.846          | 12.688         | 541.66         |
| Gain (performance) |                | ↑ <b>0.319</b> %     | -              | -              | -              | -              |
| Gain (efficiency)  |                | -                    | <b>100.31%</b> | ↓ <b>1.3</b> × | ↓ <b>1.3</b> × | ↓ <b>1.3</b> × |

Table 4: *TopicBERT* for document classification (macro-F1) for AGnews dataset. *Rtn*: Retention in *F1* vs *BERT*;  $T_{epoch}$ : average epoch time (in hours); *T*:  $T_{epoch} \times 15$  epochs;  $CO_2$ : Carbon footprint in *gram eq.* (Power consumption  $\times T \times$  Carbon produced by power grid); **bold**: Best (fine-tuned BERT-variant) in column; underlined: Most efficient *TopicBERT-x* vs *BERT*; Gain (performance): *TopicBERT-x* vs *BERT*; Gain (efficiency): underlined vs *BERT*

*icBERT* achieves: (a) a gain of 0.3% in *F1* (*performance*) compared to *BERT*, and (b) a significant speedup of  $1.3 \times$  over *BERT* while retaining (*Rtn*) 100% of *F1* (*performance*) of *BERT* at the same time. This gain arises due to the improved document understanding using complementary topical semantics, via NVDM, in *TopicBERT* and its energy efficient versions.

## E TopicDistilBERT vs DistilBERT

Table 5 reports scores of *TopicDistilBERT* vs *DistilBERT* for two datasets (Reuters8 and 20NS). We follow the similar schemes of sequence lengths (512, 256 and 128) to evaluate the performance of the (a) complementary learning via *TopicDistilBERT-512* vs *DistilBERT*, and (b) efficient learning via *TopicDistilBERT*-{256, 128} vs *DistilBERT*.

For Reuters8 in complementary setup, *TopicDistilBERT-512* achieves a gain (0.941 vs 0.934) in *F1* over *DistilBERT*. In the efficient setup, *TopicDistilBERT-256* achieves a significant speedup of  $1.5 \times$  ( $1.5 \times$ , i.e.,  $\sim 50\%$  reduction in  $CO_2$ ) in fine-tuning while retaining (*Rtn*) 100.96% of *F1* of *DistilBERT*.

For 20NS in complementary setup, *TopicDistilBERT-512* achieves a gain (0.820 vs 0.816) in *F1* over *DistilBERT*. In the efficient setup, *TopicDistilBERT-256* achieves a speedup of  $1.6 \times$  ( $1.6 \times$ , i.e.,  $\sim 60\%$  reduction in  $CO_2$ ).

Additionally, *TopicBERT-512* exceeds *Distil-*

|           | Models                     | Reuters8 (news domain)              |                |                        |                        |                        | 20NS (news domain)                  |                |                        |                        |                        |
|-----------|----------------------------|-------------------------------------|----------------|------------------------|------------------------|------------------------|-------------------------------------|----------------|------------------------|------------------------|------------------------|
|           |                            | $F1$                                | $Rtn$          | $T_{epoch}$            | $T$                    | $CO_2$                 | $F1$                                | $Rtn$          | $T_{epoch}$            | $T$                    | $CO_2$                 |
| baselines | <i>CNN</i>                 | $0.852 \pm 0.000$                   | 91.123%        | 0.007                  | 0.340                  | 14.51                  | $0.786 \pm 0.000$                   | 95.504%        | 0.109                  | 1.751                  | 74.76                  |
|           | <i>DistilBERT</i>          | $0.934 \pm 0.003$                   | 100.00%        | 0.129                  | 1.938                  | 82.75                  | $0.816 \pm 0.005$                   | 100.000%       | 0.313                  | 4.700                  | 200.69                 |
| proposals | <i>TopicDistilBERT-512</i> | $0.941 \pm 0.007$                   | 100.75%        | 0.132                  | 1.976                  | 84.37                  | <b><math>0.820 \pm 0.000</math></b> | <b>100.49%</b> | 0.320                  | 4.810                  | 205.38                 |
|           | <i>TopicDistilBERT-256</i> | <b><math>0.943 \pm 0.006</math></b> | <b>100.96%</b> | <b>0.085</b>           | <b>1.272</b>           | <b>54.31</b>           | $0.802 \pm 0.000$                   | <u>98.284%</u> | <b>0.190</b>           | <b>2.850</b>           | <b>121.69</b>          |
|           | <i>TopicDistilBERT-128</i> | $0.911 \pm 0.012$                   | 97.573%        | 0.096                  | 1.444                  | 61.66                  | $0.797 \pm 0.000$                   | 97.671%        | 0.387                  | 5.800                  | 247.66                 |
|           | Gain (performance)         | $\uparrow 0.964\%$                  | -              | -                      | -                      | -                      | $\uparrow 0.490\%$                  | -              | -                      | -                      | -                      |
|           | Gain (efficiency)          | -                                   | <b>100.96%</b> | $\downarrow 1.5\times$ | $\downarrow 1.5\times$ | $\downarrow 1.5\times$ | -                                   | <b>98.284%</b> | $\downarrow 1.6\times$ | $\downarrow 1.6\times$ | $\downarrow 1.6\times$ |

Table 5: *TopicDistilBERT* vs *DistilBERT* for document classification (macro-F1) in complementary (*TopicDistilBERT*-512) and efficient (*TopicDistilBERT*-{256, 128}) learning setup. Here,  $Rtn$ : Retention in  $F1$  vs *BERT*;  $T_{epoch}$ : average epoch time (in hours);  $T$ :  $T_{epoch} \times 15$  epochs;  $CO_2$ : Carbon footprint in *gram eq.* (Power consumption  $\times T \times$  Carbon produced by power grid); **bold**: Best (fine-tuned *DistilBERT*-variant) in column; underlined: Most efficient *TopicDistilBERT*- $x$  vs *DistilBERT*; Gain (performance): *TopicDistilBERT*- $x$  vs *DistilBERT*; Gain (efficiency): underlined vs *DistilBERT*

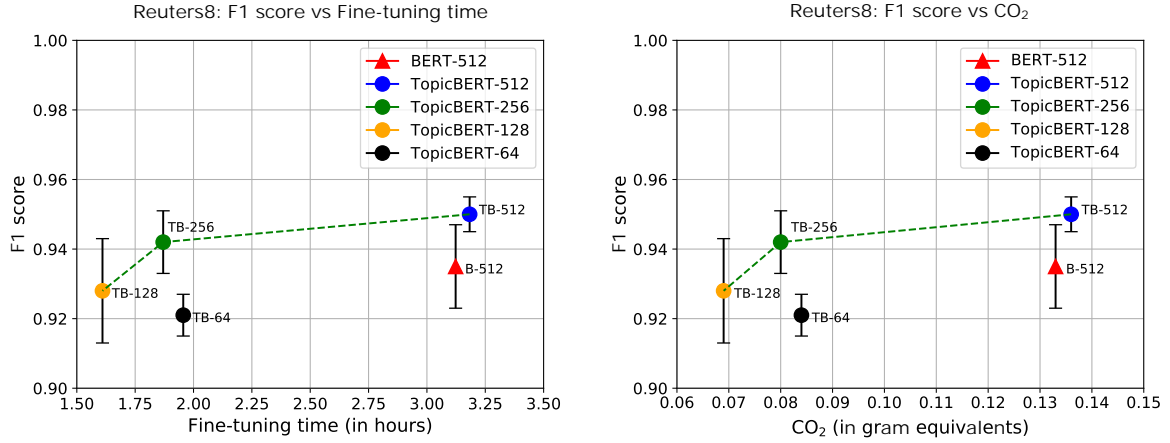

Figure 1: Pareto frontier analysis of Reuters8 dataset:  $F1$  score vs Fine-tuning time (left) and  $F1$  score vs  $CO_2$  (carbon footprint) (right). Here green dashed line represents Pareto frontier connecting optimal solutions

*BERT* in  $F1$  for the two datasets. At  $p = 4$ , *TopicDistilBERT*-128 does not achieve expected efficiency perhaps due to saturated GPU-parallelization (a trade-off in decreasing sequence length and increasing #batches) and therefore, we do not partition further.

Overall, *TopicDistilBERT*- $x$  achieves gains in: (a) *performance*: 0.964%, and 0.490% in  $F1$  for Reuters8 and 20NS, respectively, and (b) *efficiency*: a speedup of  $1.55\times$  ( $\sim 55\%$ ) and thus, a reduction of  $\sim 55\%$  in  $CO_2$  over 2 datasets while retaining 99.6% of  $F1$  compared to *DistilBERT* baseline model.

It suggests that the topical semantics improves document classification in *TopicDistilBERT* (and *TopicBERT*) and its energy-efficient variants. Based on our two extensions: *TopicBERT* and *TopicDistilBERT*, we assert that our proposed approaches of complementary learning (fine-tuning)

are *model agnostic* of *BERT* models.

## F Experimental Analysis

### F.1 Optimal sequence length (Pareto Analysis)

As shown in Table 3 (in paper content), gains in *TopicBERT* has been analyzed on two different fronts: (a) gain on the basis of *performance* ( $F1$  score), and (b) gain on the basis of *efficiency* (Fine-tuning time or  $CO_2$ ). Figure 1 shows the following Pareto frontier analysis plots for Reuters8 dataset: (a)  $F1$  score vs Fine-tuning time (left), and (b)  $F1$  score vs  $CO_2$  (right) to find the optimal solution that balances both fronts. Observe that the *TopicBERT*-512 outperforms all other *TopicBERT* variants and *BERT* baseline (B-512) in terms of *performance* i.e.,  $F1$  score. However, *TopicBERT*-256 outperforms *BERT*-512 in terms of both, *perform-*

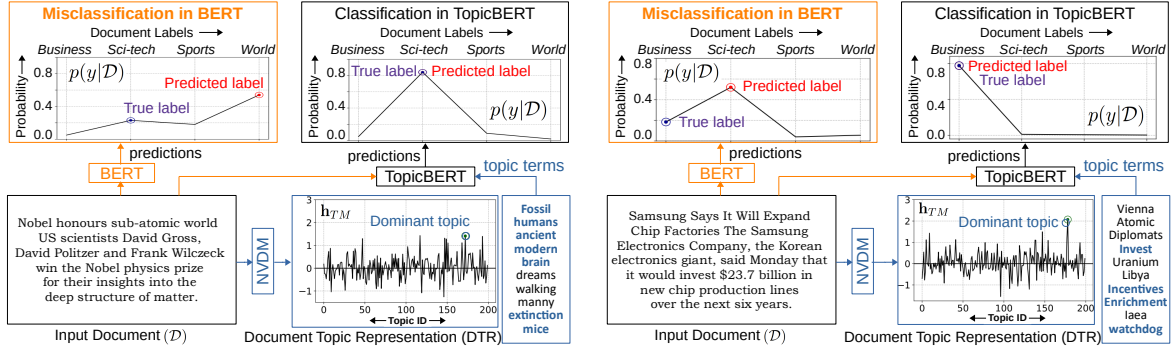

Figure 2: Interpretability analysis of document classification for AGnews dataset (for 2 input documents): Illustration of document misclassification by *BERT* model and correct classification by *TopicBERT* explained by the top key terms of dominant topic in DTR.

mance (*F1* score) and efficiency (Fine-tuning time or *CO*<sub>2</sub>). Therefore, *TopicBERT*-256 represents the optimal solution with optimal sequence length of 256 for Reuters8 dataset.

## F.2 Interpretability in TopicBERT

To analyze the gain in performance (*F1* score) of *TopicBERT* vs *BERT*, Figure 2 shows document label misclassifications due to *BERT* model. However, *TopicBERT* model is able to correctly predict the labels using document topic representation (DTR) which explains the correct predictions by the top key terms of the dominant topic discovered.
